# Supplementary material for: Statistical mechanics far from equilibrium: prediction and test for a sheared system
Source: arXiv:0911.0830 source file (2009-11-04)
Supplement: Supplementary file 1 [file supplement.pdf]

# Supplement

R. M. L. Evans, R. A. Simha, A. Baule and P. D. Olmsted

9 September 2009

## 1 Additional data

Further data, giving independent tests of the predicted relationships are shown in the figure, for parameter values different from those presented in the Letter.

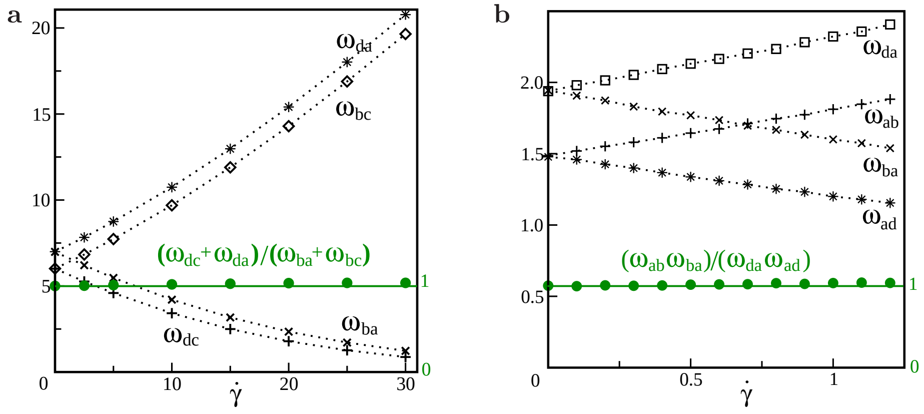


Figure 1: (a) Test of the prediction $\omega_{ba} + \omega_{bc} = \omega_{da} + \omega_{dc}\ \forall\ \dot{\gamma}$ with noise strengths $\sigma = 20$. The left-hand ordinate measures rates, using the same units as the abscissa, while the right-hand ordinate measures the dimensionless ratio. (b) Test of the predicted relationship $\omega_{ab}\,\omega_{ba} = \omega_{ad}\,\omega_{da}\ \forall\ \dot{\gamma}$, with noise strength $\sigma = 10$.

## 2 Occupancies of microstates in the driven steady state

We derive in this supplement a relation for the occupancies of microstates in the driven steady state of a complex fluid subjected to shear by a non-equilibrium reservoir of surrounding fluid as described in the accompanying paper.

We consider a set of phase-space trajectories, microscopically describing the possible evolutions of a fluid over some long duration during which it may acquire some trajectory-dependent shear strain $\gamma$. In the *prior* set of trajectories, we put no constraint on the possible values of $\gamma$, so that prior set describes an equilibrium ensemble, for which the fluctuating values of $\gamma$ are mostly small, and average to zero. The driven ensemble is then derived from the *prior* set by imposing a *posterior* constraint on the distribution of $\gamma$ values. Since all trajectories suffer from initial transients, properties of the steady state must be obtained by interrogating features in the middle of the trajectories, i.e., at or near time $t = 0$ for an ensemble of trajectories defined on the time-interval $[-\tau, \tau]$ with large $\tau$.

Let $(a)_t$ denote the fact that the system passes through microstate $a$ at time $t$. Hence $(a)_t$ represents a statement, that may be true or false for a given trajectory. Let ${}_{t_1}[\,2\gamma\,]_{t_2}$ denote the statement (also true for only a subset of trajectories) that the net strain accumulated in the system between time $t_1$ and $t_2$ is $2\gamma$. Let us imagine time to be discretized into infinitessimal intervals of duration $\Delta t$. Then, in this notation, an equilibrium transition rate is given by

$$\omega_{ab}^{\mathrm{eq}}\Delta t = \Pr\left((a)_0, (b)_{\Delta t}\,|\,(a)_0\right) \qquad (1)$$

where $\Pr\left((a)_0,(b)_{\Delta t}\,|\,(a)_0\right)$ is the conditional probability that a randomly selected trajectory passes through two particular microstates $a$ and $b$ on the consecutive time-steps at $t=0$ and $t=\Delta t$ respectively, given that it is in state microstate $a$ at $t=0$. Similarly, the transition rate in the driven ensemble for which the system's net accumulated shear strain is constrained (termed in "microcanonical flux ensemble" in Ref. [1]) is given by

$$\omega_{ab}^{\rm eq}\Delta t = \lim_{\tau\to\infty} \Pr\left((a)_0,(b)_{\Delta t}\,|\,(a)_{0,-\tau}\,[\,2\gamma\,]_\tau\right). \tag{2}$$

Let us conjecture that, in the steady state, any conditional probablility $\Pr(\,X\,|\,Y,{}_{-\tau}[\,2\gamma\,]_\tau)$ is dominated by trajectories with the macroscopic strain $2\gamma$ equally divided between the macroscopic intervals $[-\tau,0\,]$ and $[0,\tau\,]$ so that

$$\Pr(X\,|\,Y,{}_{-\tau}[\,2\gamma\,]_\tau) \xrightarrow[\tau\to\infty]{\gamma=\dot\gamma\tau} \Pr(X\,|\,Y,{}_{-\tau}[\,\gamma\,]_0,{}_0[\,\gamma\,]_\tau)$$

and hence

$$\omega_{ab}^{\rm eq}\Delta t = \lim_{\tau\to\infty} \Pr((b)_{\Delta t}\,|\,(a)_0,{}_{-\tau}[\,\gamma\,]_0,{}_0[\,\gamma\,]_\tau). \tag{3}$$

However, the probability of any events at or after time 0 is independent of events before time 0 given that the system is in microstate $a$ at time 0. Hence, the dependence on ${}_{-\tau}[\,\gamma\,]_0$ can be dropped. So,

$$\omega_{ab}^{\rm eq}\Delta t = \lim_{\tau\to\infty} \Pr\left(\,(b)_{\Delta t}\,|\,(a)_0,{}_0[\,\gamma\,]_\tau\right) \tag{4}$$

consistent with the definition used in Ref. [1]. i.e., the probability of a transition can legitimately be conditioned on the subsequent shear strain only, irrespective of whether the system was flowing before the transition. However, to find a general formula for the *occupancies* (as opposed to transition rates), no such simplification exists; the entire trajectory in the interval $[-\tau,\tau]$ must be properly constrained (as shown below) in order to avoid the influence of non-steady-state transients.

The occupancy of a microstate $a$ is given by

$$f^{\rm eq}(a) = \Pr\big((a)_0\big) \tag{5}$$

$$\text{and}\qquad f^{\rm dr}(a) = \lim_{\tau\to\infty}\Pr\big((a)_0\,|\,{}_{-\tau}[\,2\gamma\,]_\tau\big) \tag{6}$$

in the equilibrium and driven ensembles respectively. Let us again appeal to the fact that, in the limit $\gamma=\dot\gamma\,\tau$ with $\tau\to\infty$, the set of trajectories with ${}_{-\tau}[\,2\gamma\,]_\tau$ is dominated by the subset with both of the properties ${}_{-\tau}[\,\gamma\,]_0$ and ${}_0[\,\gamma\,]_\tau$. Hence

$$\begin{aligned} f^{\rm dr}(a) &= \lim_{\tau\to\infty}\Pr\big((a)_0\,|\,{}_{-\tau}[\,\gamma\,]_0,{}_0[\,\gamma\,]_\tau\big) \\ &= \lim_{\tau\to\infty}\Pr\big({}_{-\tau}[\,\gamma\,]_0,{}_0[\,\gamma\,]_\tau\,|\,(a)_0\big)\frac{\Pr\big((a)_0\big)}{\Pr\big({}_{-\tau}[\,\gamma\,]_0,{}_0[\,\gamma\,]_\tau\big)} \end{aligned} \tag{7}$$

where the second line follows from Bayes' theorem. The factors on the RHS of the above equation can be re-written as follows. Firstly, in a Markovian process, given a particular microstate at time 0, the probabilities of events before and after, ${}_{-\tau}[\,\gamma\,]_0$ and ${}_0[\,\gamma\,]_\tau$, are independent of each other, so that

$$\Pr\big({}_{-\tau}[\,\gamma\,]_0,{}_0[\,\gamma\,]_\tau\,|\,(a)_0\big) = \Pr\big({}_{-\tau}[\,\gamma\,]_0\,|\,(a)_0\big)\Pr\big({}_0[\,\gamma\,]_\tau\,|\,(a)_0\big). \tag{8}$$

Secondly, in the absence of that conditioning, in the equilibrium ensemble, and for $\tau$ greatly exceeding any correlation time,

$$\Pr\big({}_{-\tau}[\,\gamma\,]_0,{}_0[\,\gamma\,]_\tau\big)\xrightarrow[\tau\to\infty]{}\Pr\big({}_{-\tau}[\,\gamma\,]_0\big)\Pr\big({}_0[\,\gamma\,]_\tau\big) \tag{9}$$

and by time translation invariance, $\Pr({}_{-\tau}[\,\gamma\,]_0)=\Pr({}_0[\,\gamma\,]_\tau)$. Hence, Eq. (7) yields

$$f^{\rm dr}(a) = f^{\rm eq}(a)\lim_{\tau\to\infty}\frac{\Pr\big({}_{-\tau}[\,\gamma\,]_0\,|\,(a)_0\big)\Pr\big({}_0[\,\gamma\,]_\tau\,|\,(a)_0\big)}{\Pr({}_0[\,\gamma\,]_\tau)^2} \tag{10}$$

Since in the equilibrium ensemble, each trajectory occurs with the same frequency as its time-reverse, we can furthermore write

$$\Pr\big({}_{-\tau}[\,\gamma\,]_0\,|\,(a)_0\big) = \Pr\big({}_0[\,-\gamma\,]_\tau\,|\,(a^\dagger)_0\big) \tag{11}$$

where $a^\dagger$ is the time-reverse of microstate $a$, i.e. with equal position co-ordinates but reversed momenta. By the same reasoning, for a system with a Hamiltonian that is spatially symmetric in the flow direction, $\Pr\left({}_0[-\gamma]_\tau\right) = \Pr\left({}_0[\gamma]_\tau\right)$. Finally, we have

$$f^{\rm dr}(a) = f^{\rm eq}(a) \cdot \lim_{\tau\to\infty} \frac{\Pr\left({}_0[\gamma]_\tau \,|\, (a)_0\right)}{\Pr\left({}_0[\gamma]_\tau\right)} \cdot \lim_{\tau\to\infty} \frac{\Pr\left({}_0[-\gamma]_\tau \,|\, (a^\dagger)_0\right)}{\Pr\left({}_0[-\gamma]_\tau\right)}. \tag{12}$$

We can further simplify Eq. (12) by again applying Bayes theorem,

$$\frac{\Pr\left({}_0[\gamma]_\tau \,|\, (a)_0\right)}{\Pr\left({}_0[\gamma]_\tau\right)} = \frac{\Pr\left((a)_0 \,|\, {}_0[\gamma]_\tau\right)}{\Pr\left((a)_0\right)} \tag{13}$$

and similarly for microstate $a^\dagger$, so that

$$f^{\rm dr}(a)\, f^{\rm eq}(a^\dagger) = \lim_{\tau\to\infty} \Pr\left((a)_0 \,|\, {}_0[\gamma]_\tau\right) \cdot \lim_{\tau\to\infty} \Pr\left((a^\dagger)_0 \,|\, {}_0[-\gamma]_\tau\right) \tag{14}$$

where $f^{\rm eq}(a^\dagger) = f^{\rm eq}(a)$. From results in [1]

$$\begin{aligned} &\lim_{\tau\to\infty} \Pr\left((a)_0 \,|\, {}_0[\gamma]_\tau\right) \;\propto\; f^{\rm eq}(a)\, e^{q_a(\nu)}, \\ \text{and} \qquad &\lim_{\tau\to\infty} \Pr\left((a^\dagger)_0 \,|\, {}_0[-\gamma]_\tau\right) \;\propto\; f^{\rm eq}(a^\dagger)\, e^{q_{a^\dagger}(-\nu)}. \end{aligned}$$

Hence, Eq. (14) relates the microstate occupancies in the driven and equilibrium ensembles by

$$\boxed{f^{\rm dr}(a) \propto f^{\rm eq}(a)\, \exp\left[\, q_a(\nu) + q_{a^\dagger}(-\nu)\,\right]} \tag{15}$$

which is found to be consistent with the occupancies found in Ref. [1] for a model with a comb-shaped state-space, for which $a^\dagger = a$ due to the absence of momentum degrees of freedom.

# References


[1] R. M. L. Evans, J. Phys. A: Math. Gen. **38**, 293 (2005).
